# Supplementary material for: Physics-inspired Generative AI models via real hardware-based noisy quantum diffusion
Source: arXiv:2505.22193 source file (2026-10-09)
Supplement: Supplementary file 1 [file supplementary.pdf]

## Supplementary Material

In Fig. S1, we show forward and backward processes for image generation implemented by the simulator *fake\_brisbane* for the digit 0 of the MNIST dataset. In Fig. S2, we illustrate the generated images for the digits 1, 2, ..., 9 of MNIST obtained with a hybrid Quantum Stochastic Walk (QSW) dynamics ( $\omega = 0.3$ ), the simulator *fake\_brisbane*, and the real IBM quantum hardware *ibm\_brisbane*.

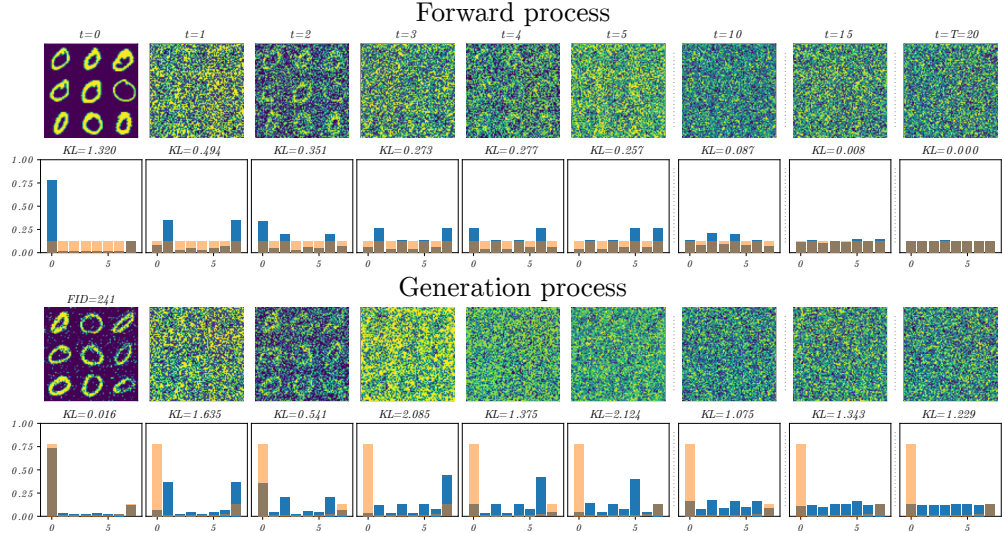

**Fig. S1:** Images generation with Quantum Walk (QW)-based Diffusion Model (DM) with noise from IBM simulator *fake\_brisbane*. We report (for selected values of  $t$ ) the evolution of 9 random samples of the real dataset in forward (first row) and 9 random generated samples in backward (third row). We also show the evolution of the pixel values distributions during forward (second row) reporting the Kullback–Leibler (KL) divergence to compare the full training dataset (blue) with the final uniform distribution (orange), and the evolution of the backward (fourth row) for an equally-sized generated dataset comparing it with the original training dataset. Finally, we calculate the FID between the original and generated dataset for  $t = 0$ .

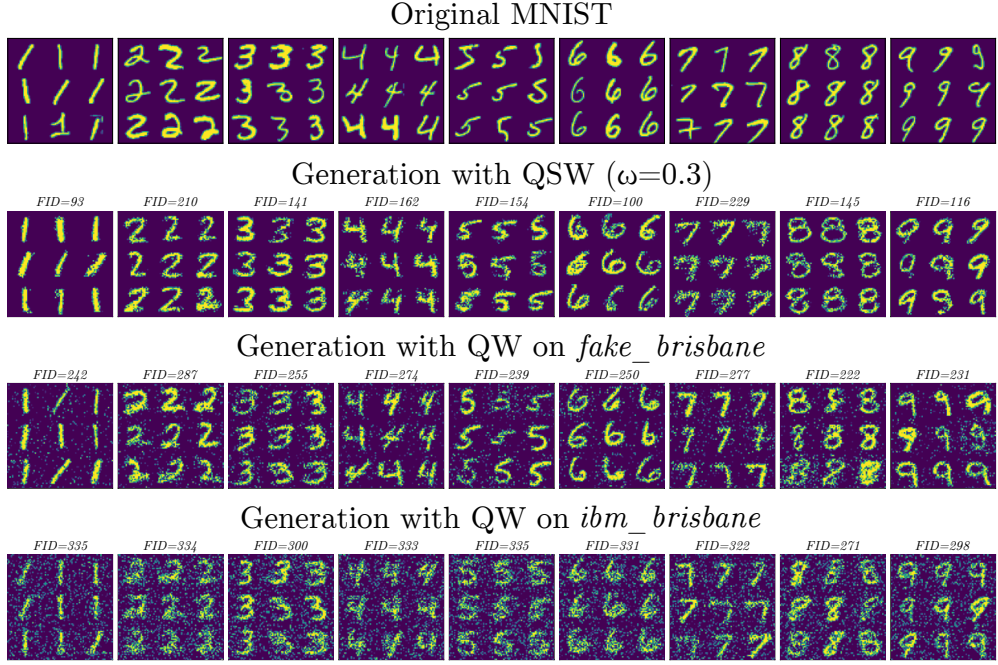

**Fig. S2:** Image generation with a hybrid QSW dynamics and a QW-based DM with noise from a simulated and a real Noisy Intermediate-Scale Quantum (NISQ) device for MNIST digit from 1 to 9 (the results for the digit 0 are already included in the main manuscript and in Fig. S1 above). We illustrate nine different samples for each handwritten digit, while in the first row the samples are taken from the original MNIST dataset. In the second row, the samples are generated via the implementation of the forward with a simulated QSW dynamics with  $\omega = 0.3$ . In the third and the fourth rows, the samples are generated using a forward implemented with QWs and executed respectively on the simulator *fake\_brisbane* and the real quantum machine *ibm\_brisbane*. We also report the FID metric values between the original full training set and a same-sized generated dataset.
